# Supplementary material for: Stochastic Combinatorial Optimization via Poisson Approximation
Source: arXiv:1211.1149 source file (2013-03-19)
Supplement: Supplementary file 1 [file appendix.tex]

\section{Discretizing small size region}
More formally, let $0\leq d\leq \e^4$ be the value such that
$
\Pr[X_b \leq d \mid X_b \leq \e^4] \cdot \e^4 \geq \E[X_b \mid X_b \leq \e^4]
$
and
$
\Pr[X_b \geq d \mid X_b \leq \e^4] \cdot \e^4 \geq \E[X_b \mid X_b \leq \e^4]
$
(note that such $d$ must exist).
For ease of presentation, we can imagine the size value $d$ being two distinguishable values,
$d_1=d-\frac{1}{\infty}$ and $d_2=d+\frac{1}{\infty}$,
and we let $d_1<d<d_2$.
The probability mass $\Pr[X_b=d]$ also consists of two parts
$\Pr[X_b=d_1]$ and $\Pr[X_b=d_2]$
and the value are so set that
$
\Pr[X_b \leq d_1 \mid X_b \leq \e^4] \cdot \e^4 = \E[X_b \mid X_b \leq \e^4]
$
and
$
\Pr[X_b \geq d_2 \mid X_b \leq \e^4] \cdot \e^4 = \E[X_b \mid X_b \leq \e^4]
$.
Therefore, in this new item, we can use value $d$ as the threshold value.
Note that
the effective profit $p_b(d)$ should also be divided accordingly:
$p_b(d_1)=p_b(d)\Pr[X_b=d_1]/ \Pr[X_b=d]$
and
$p_b(d_2)=p_b(d)\Pr[X_b=d_2]/ \Pr[X_b=d]$.
